# Supplementary material for: Super-critical accretion of medium-weight seed black holes in gaseous proto-galactic nuclei
Source: arXiv:2204.10330 source file (2022-12-09)
Supplement: Supplementary file 1 [file appendix.tex]

  %\begin{figure*}
 
%     \centering
%     \includegraphics [scale=0.25]{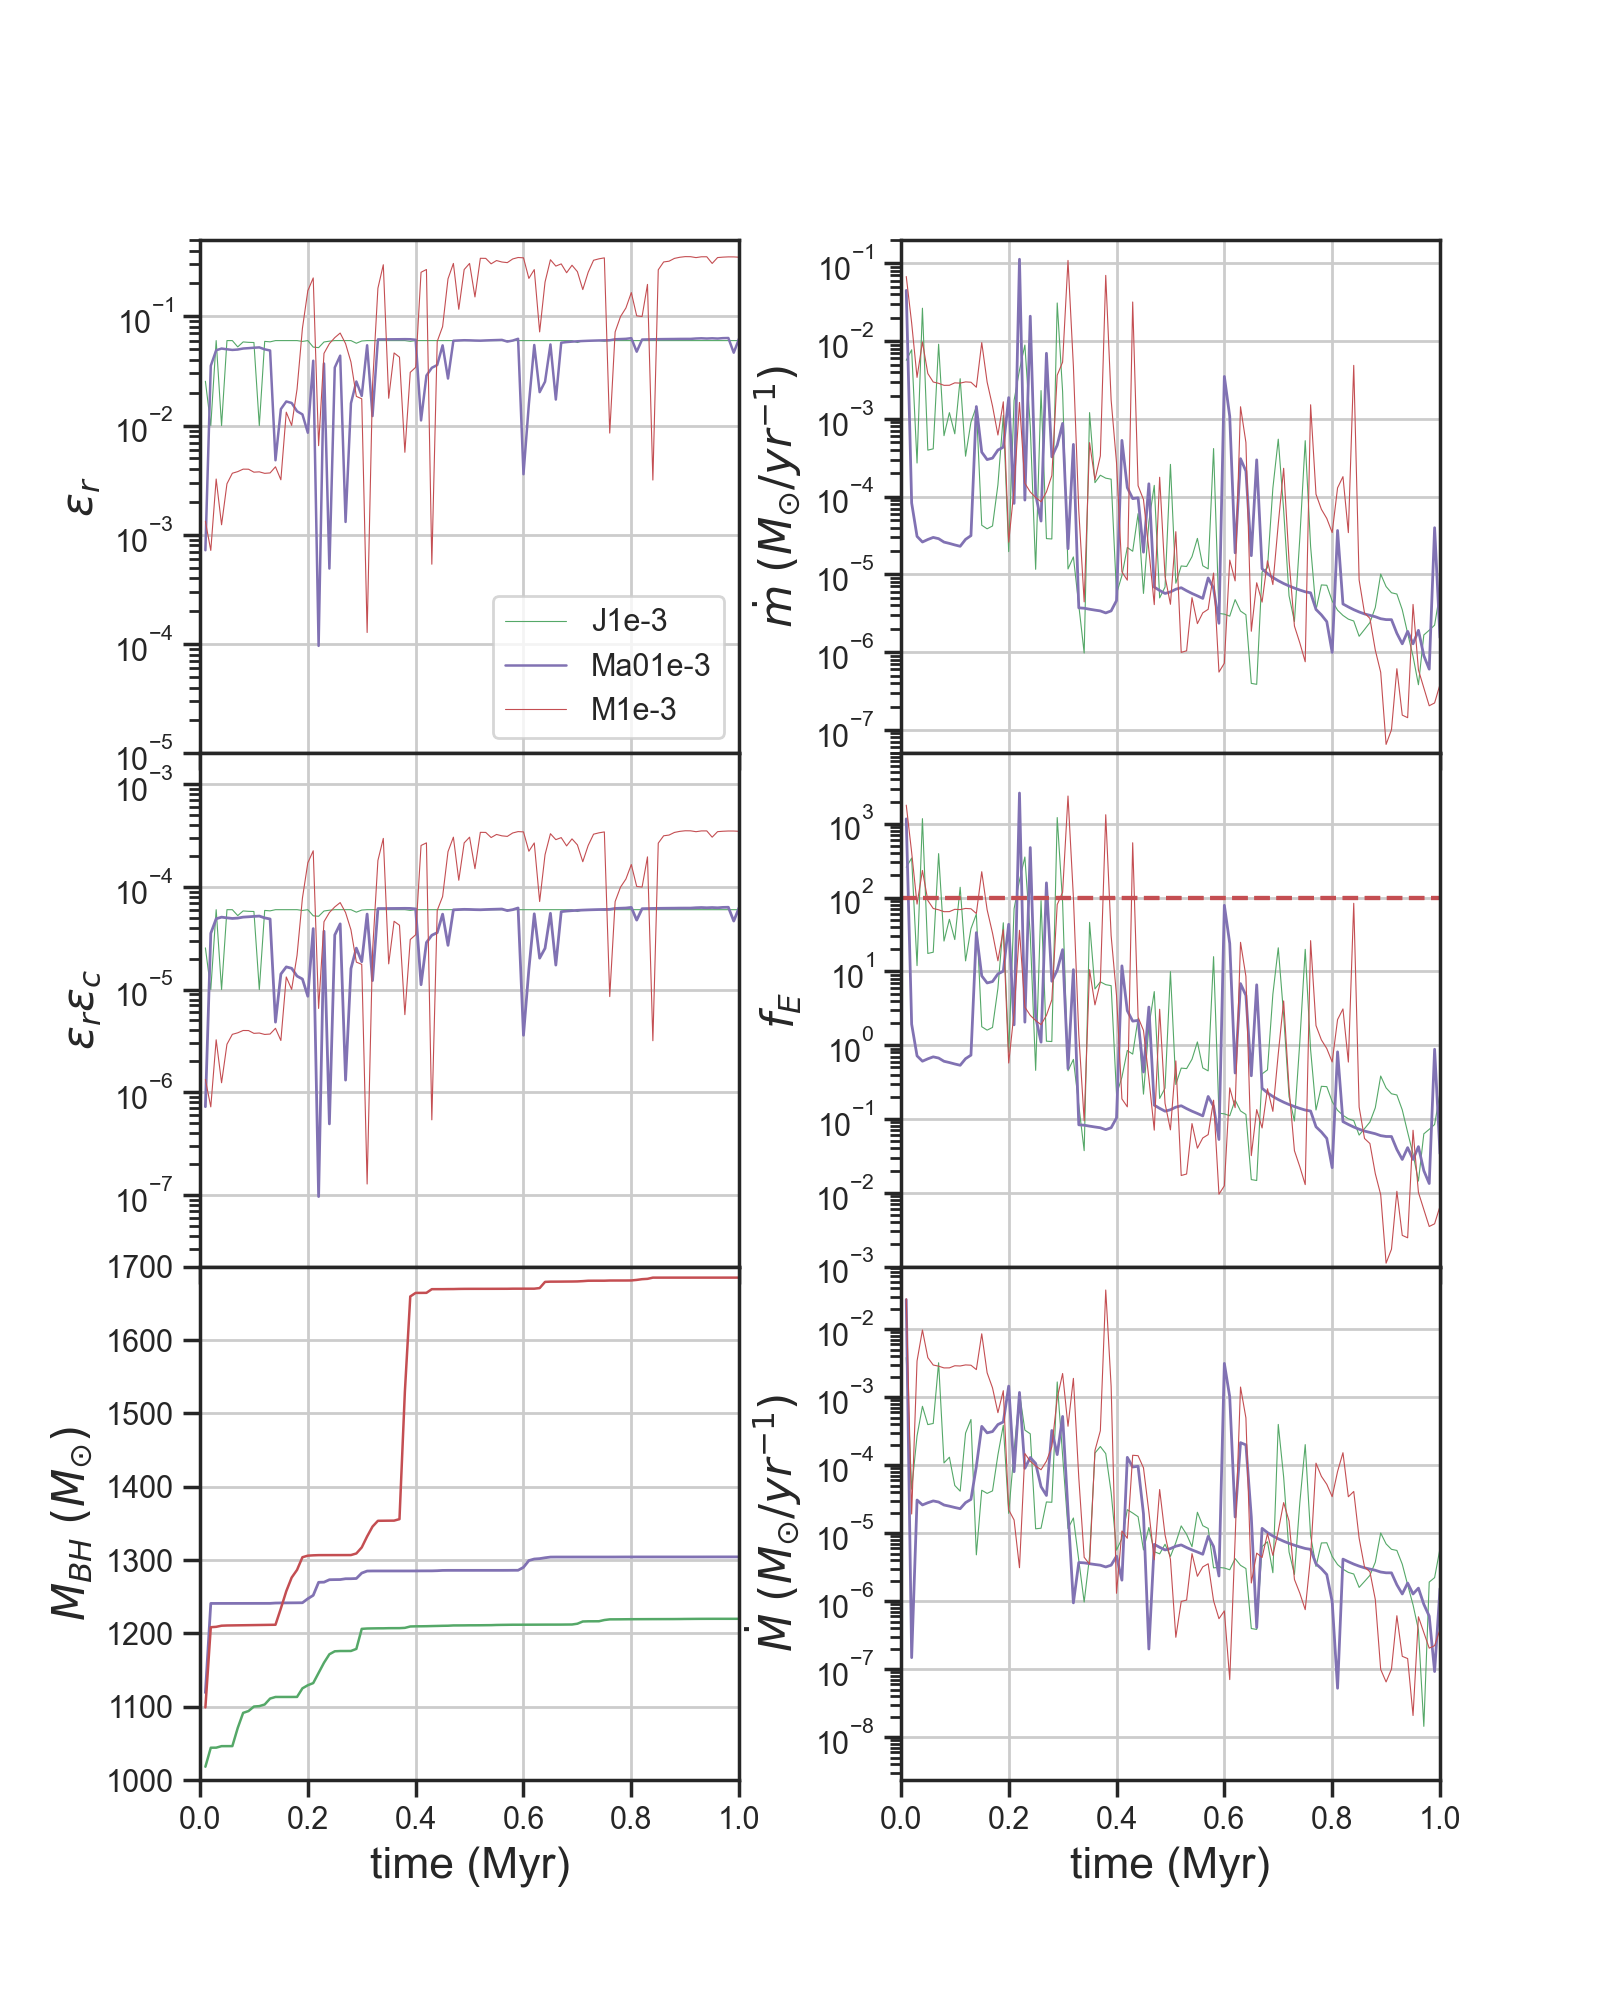}
 %    \caption{Same as Fig. \ref{fig:1e3} but for Madau model with spin parameter $a=0$.}
%     \label{fig:ma1e-3}
% \end{figure*}
 
 %\begin{figure*}
    
 %    \centering
 %    \includegraphics [scale=0.49]{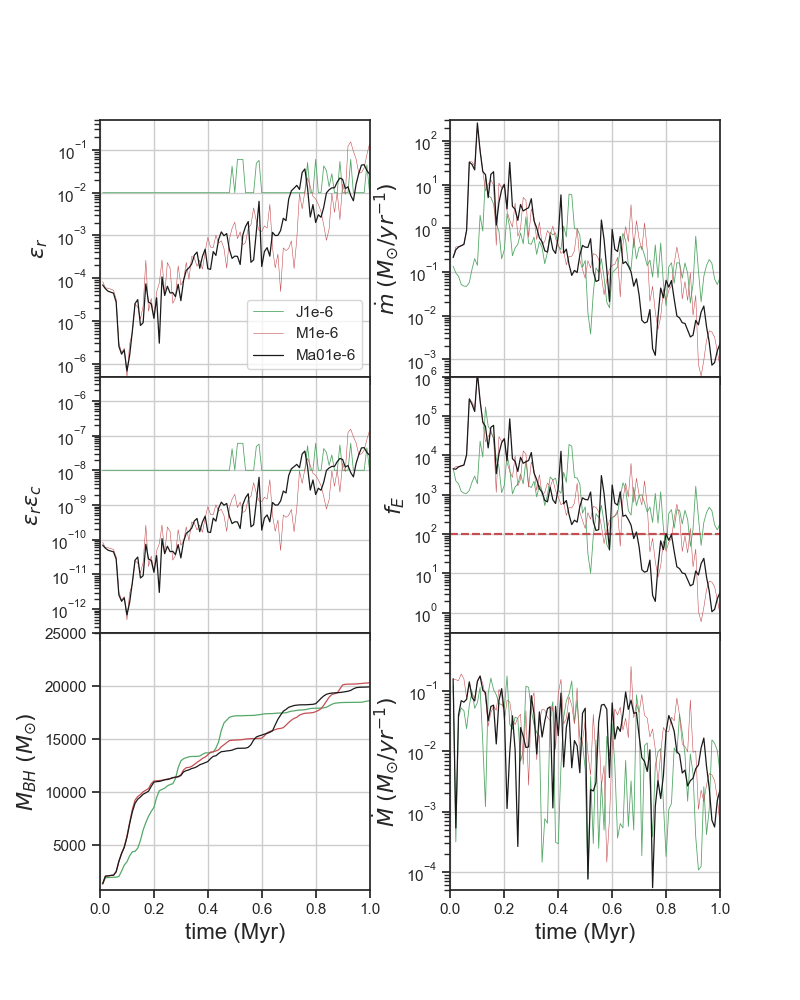}
 %    \caption{Same as Fig. \ref{fig:1e-6} but for Madau model with spin parameter $a=0$.}
 %    \label{fig:ma1e-6}
% \end{figure*}
 
 %\begin{figure*}
  
%    \centering
 %   \includegraphics [scale=0.42]{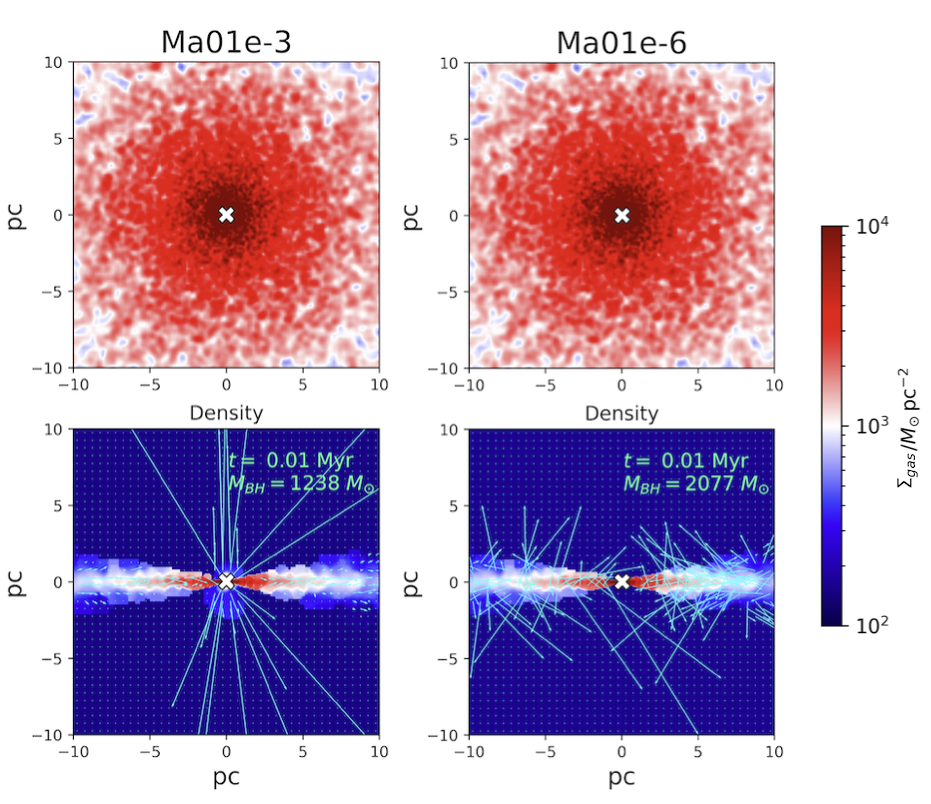}
%    \includegraphics [scale=0.4]{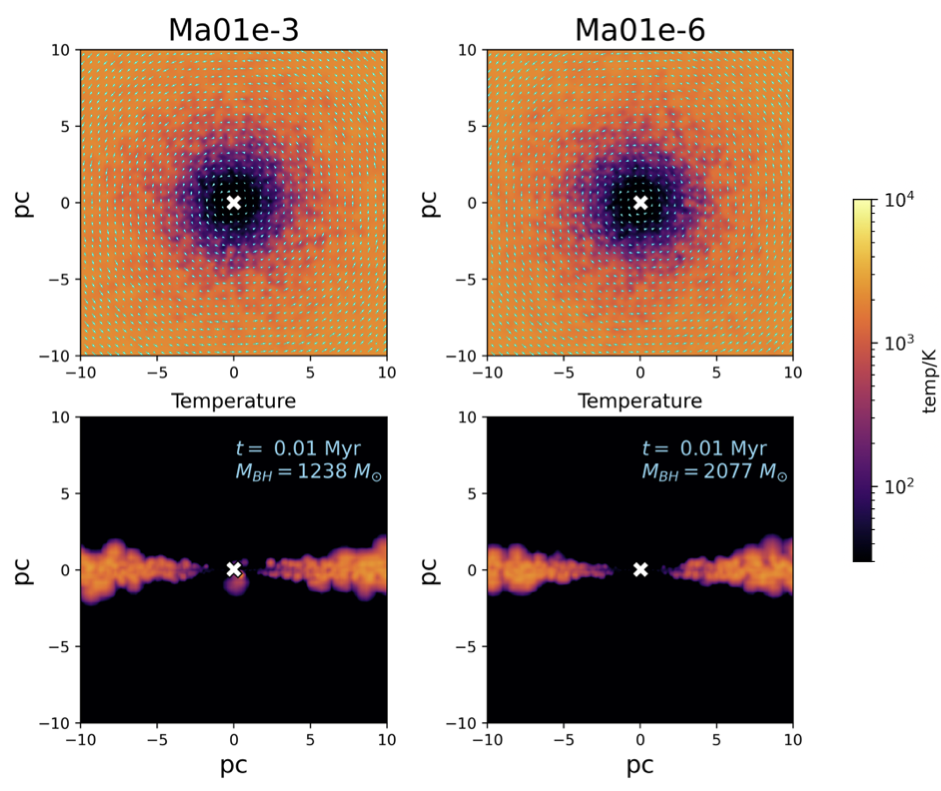}

%    \caption{Gas density (upper 4 panels) and temperature (lower 4 panels) profiles of the disk at $t=0.01$ Myr, for the two runs, Ma01e-3 (left colum) and Ma01e-6 (right column). Odd and even rows show a face-on and edge-on view of the disk, respectively. Cyan arrows indicate the direction and magnitude of the velocity flows. The white crosses mark the positions of the BHs.}
%    \label{fig:snapa01}
%\end{figure*}

 %\begin{figure*}
 %   \centering
 %   \includegraphics [scale=0.48]{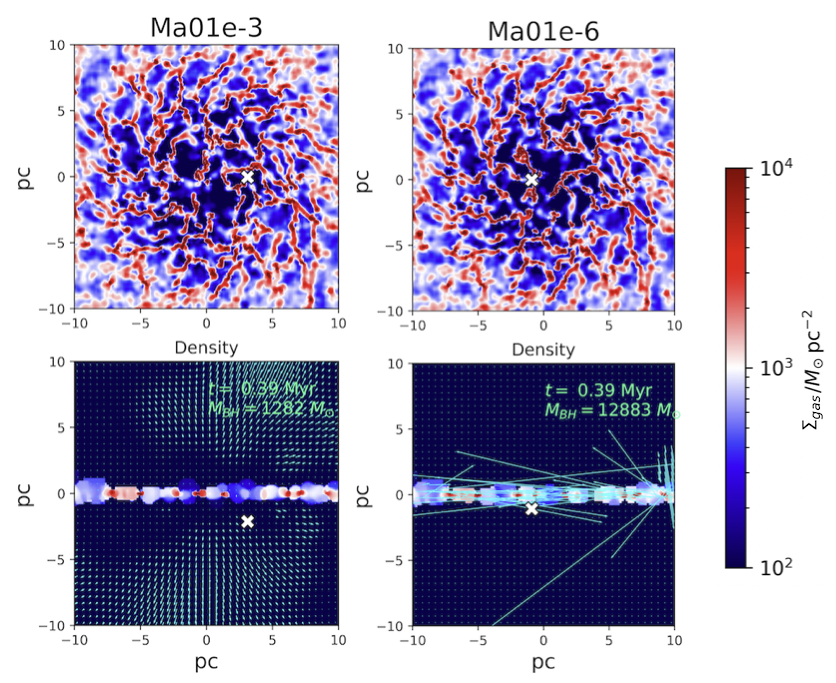}
%    \includegraphics [scale=0.42]{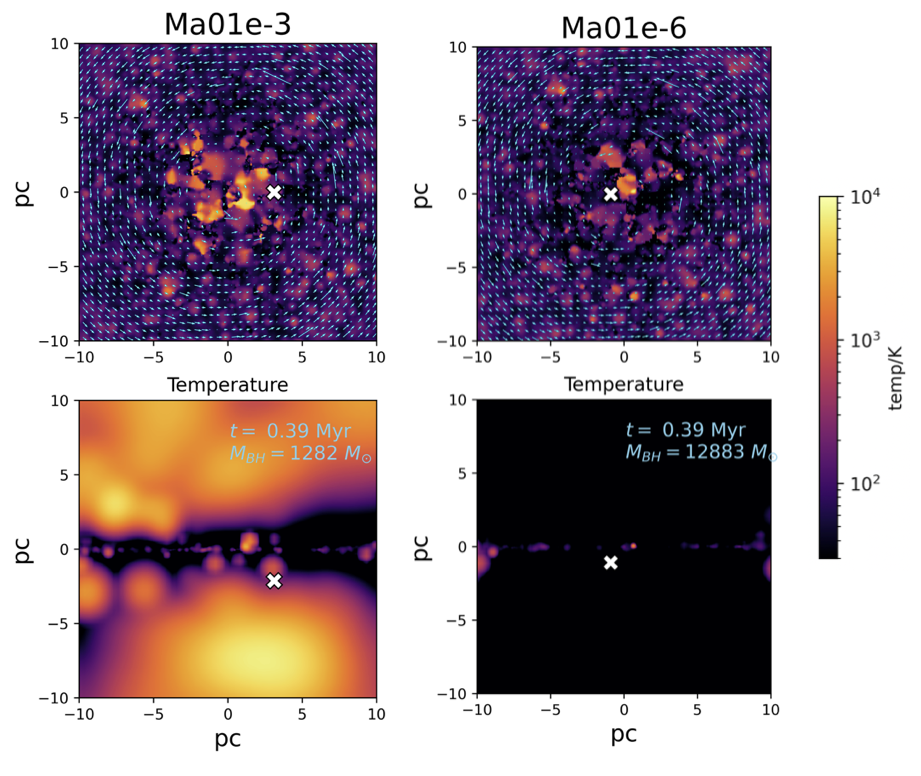}

 %   \caption{Same as Fig. \ref{fig:snapa01} but for $t=0.39$ Myr.}
%    \label{fig:snapa02}
%\end{figure*}

\begin{figure}
    \centering
     \includegraphics [scale=0.15]{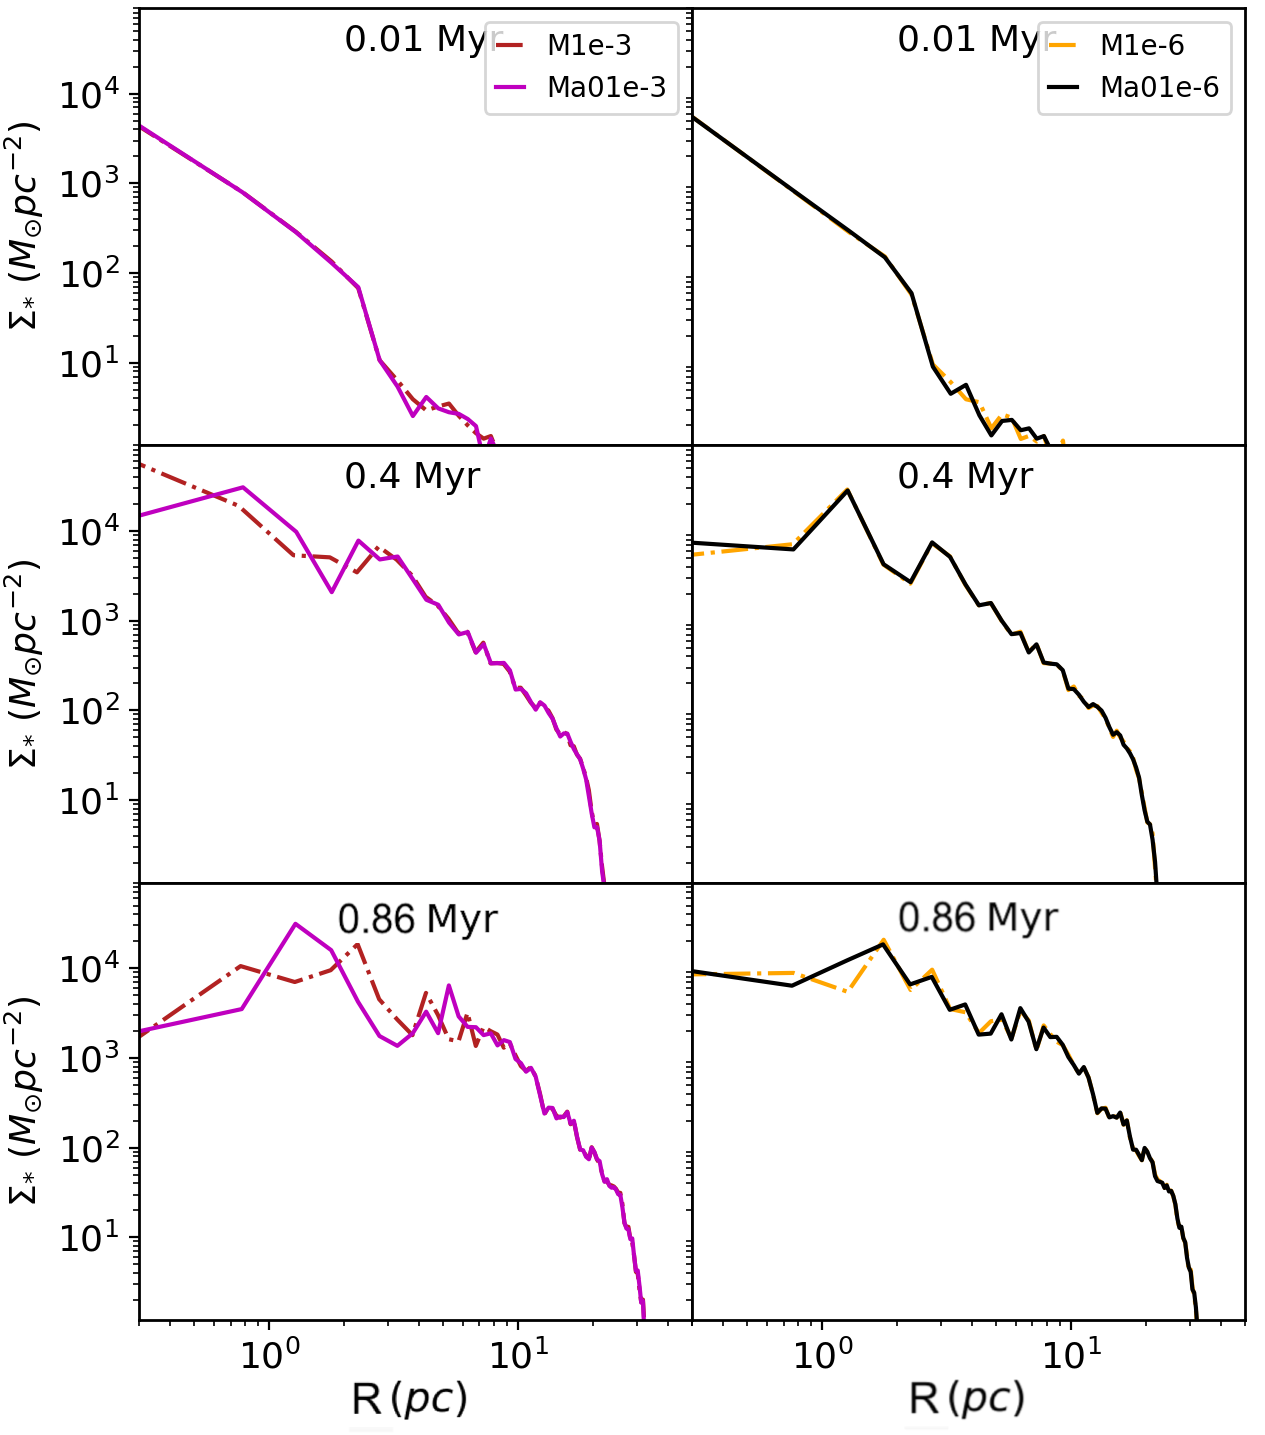}
     \includegraphics [scale=0.15]{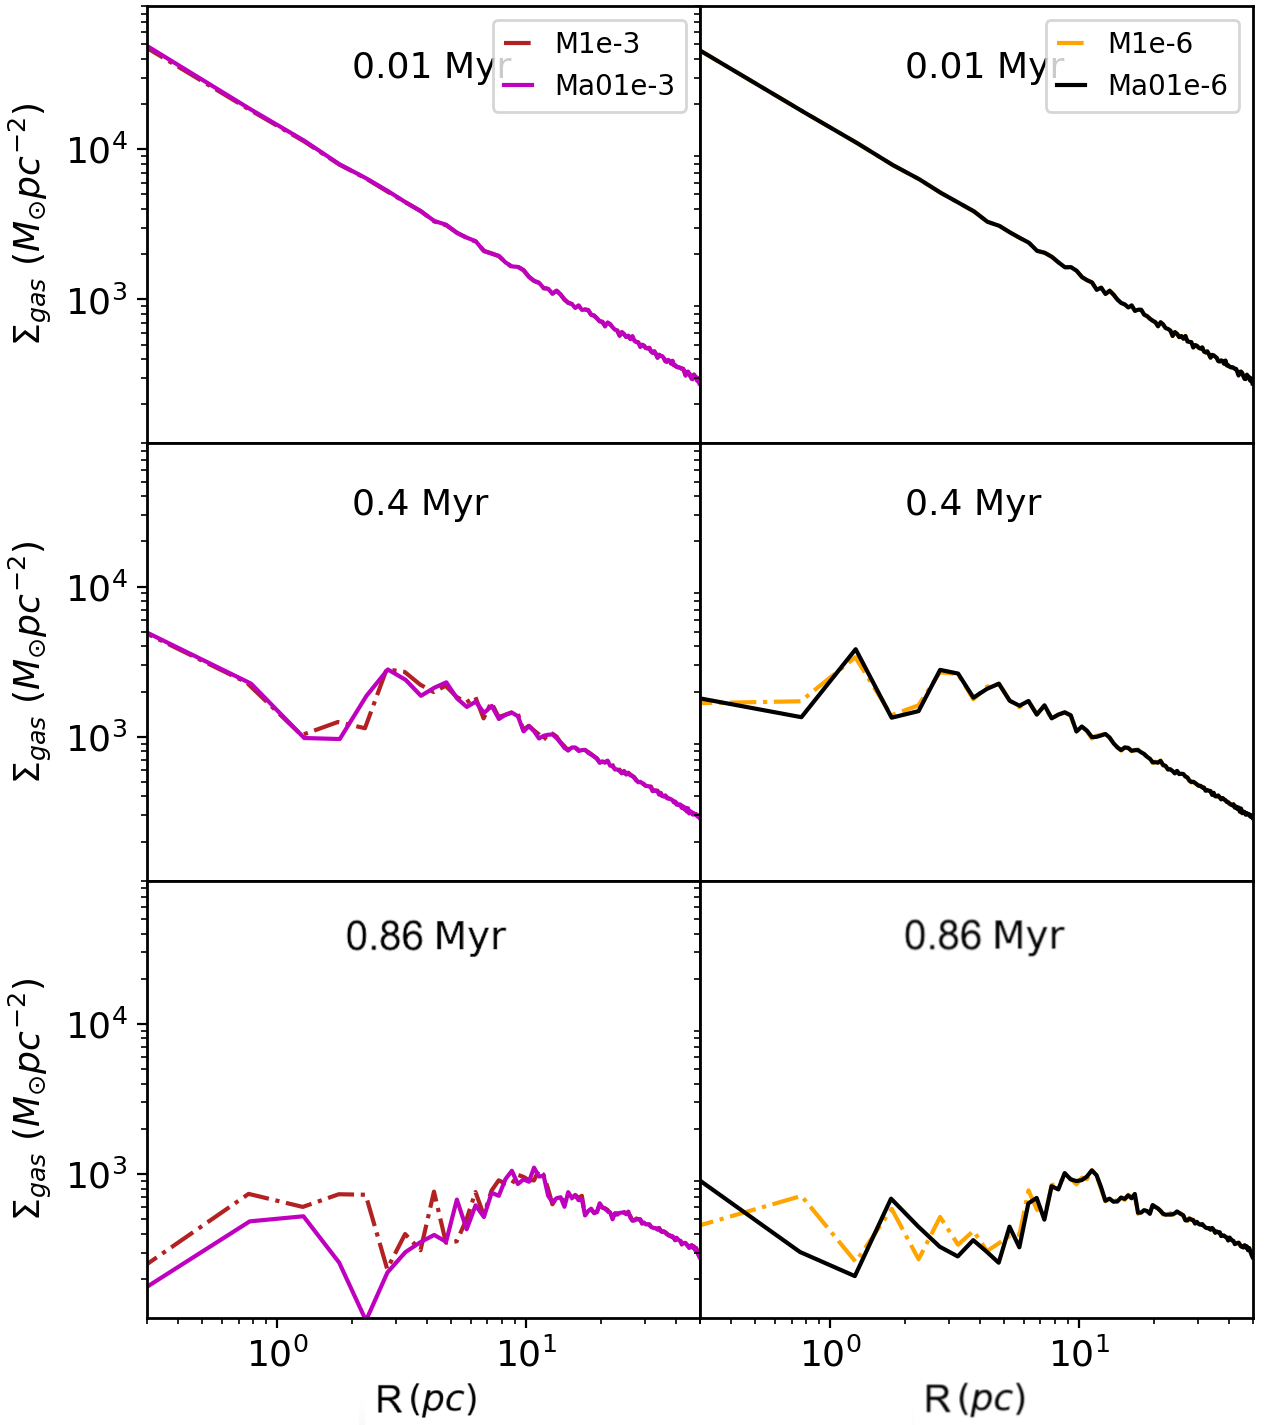}
    \caption{Same as Figs. \ref{fig:Sigmadens}, \ref{fig:Stardens} but showing the radial profile of the gas and stellar surface density for runs M1e-6, M1e-3 with $a=0$.}
    \label{fig:densa0}
\end{figure}

\begin{figure}
    \centering
    \includegraphics [scale=0.16]{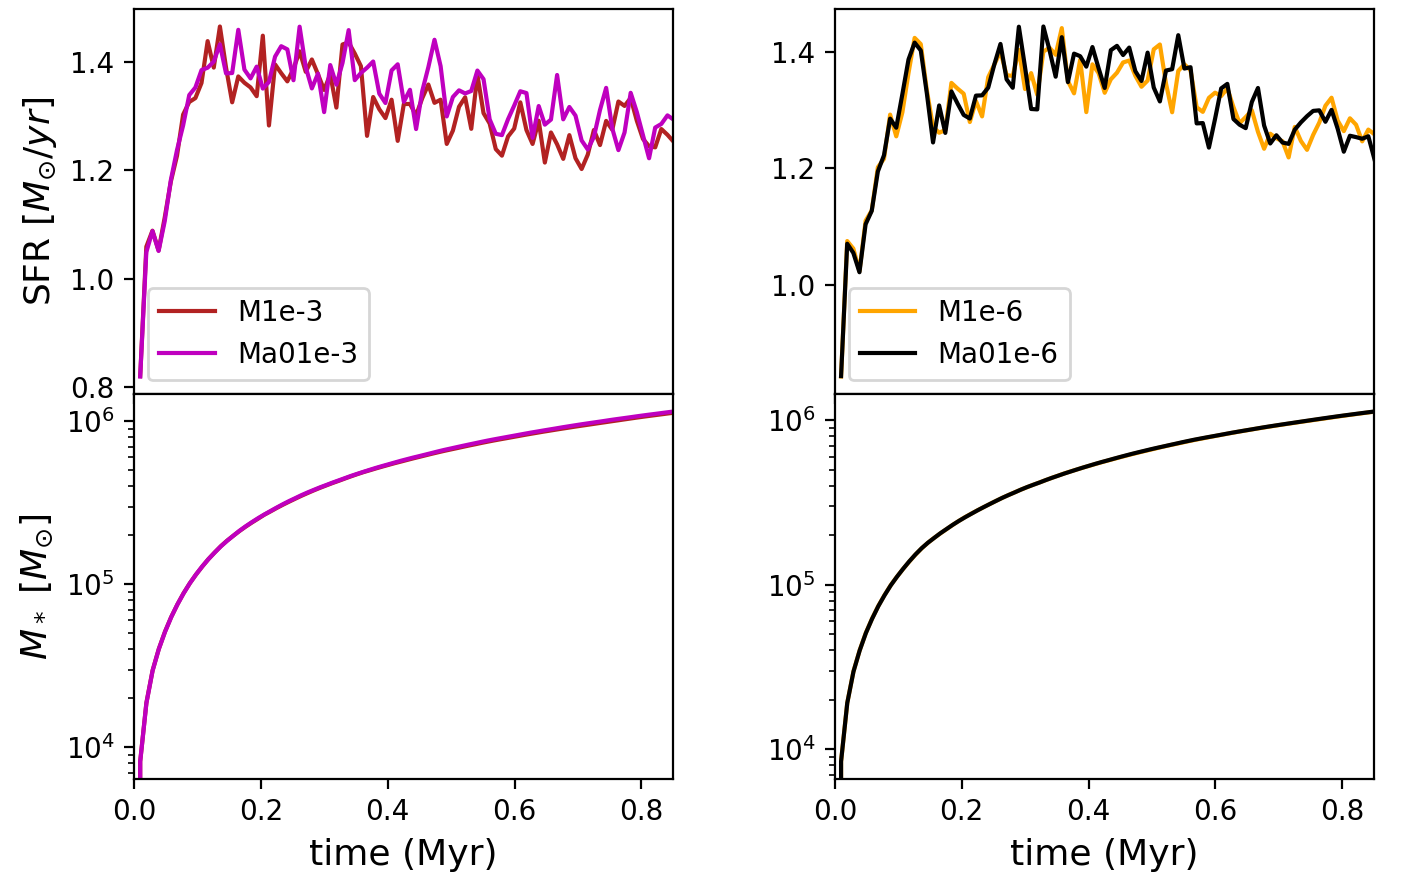}
    \caption{Same as Fig. \ref{fig:SFMstar} but for runs M1e-6, M1e-3 with $a=0.99$, and Ma01e-6, Ma01e-3 with $a=0$.}
    \label{fig:SFMstar}
\end{figure}

\subsection{Slim disk model and no-spinning BH}
\label{subsection:nospin}
In this section we report the results of two additional simulations, Ma01e-3 and Ma01e-6, where we have assumed $\epsilon_c = 10^{-3}$ and $10^{-6}$ and the value of the radiative efficiency predicted by the slim disk model for non-spinning BHs. As shown by Fig. \ref{fig:jiangmadau}, with this choice the Jiang and slim disk model predict the same value of $\epsilon_r$ when $f_E < 1$.

%In Sections \ref{subsection:Maximal} and \ref{subsection:Maximal} we have discussed different BH accretion mechanisms in the Madau and Jiang models, when a maximal and minimal feedback model is adopted, and respectively when $\epsilon_c=10^{-3}$ and $\epsilon_c=10^{-6}$. However, in the Madau model, depending on the spin of the BH, differences of $\epsilon_r$ can be enhanced, in particular for low $f_E$. 

The dashed lines in Fig. \ref{fig:1e3} show the results of Ma01e-3 (left panel), Ma01e-5 (central panel), and Ma01e-6 (right panel). Comparing Ma01e-3 with M1e-3, red dashed and solid lines, it is clear that the spin of the BH has a large impact on the time evolution of the gas accretion rate and - consequently - on the BH mass growth. At the very beginning of the simulation, the BH mass growth in model Ma01e-3  follows the same behaviour of model M1e-3. Indeed, at the very beginning gas accretion is highly SE and in this regime $\epsilon_r$ has a very small dependence on the spin in slim disk model. %This is also clear from the left column of 
%Fig. \ref{fig:snapa01}, where we show the gas density and temperature maps of the disk at $t = 0.01$ Myr. The results are almost identical to what we find for M1e-3. %(see the left column of Fig. \ref{fig:snap1e3}).
{\bf FEDE: Ho rimosso le snapshots per queste runs, con reltivi commenti su gas density and temperature maps.}
However, after a few time steps, the accretion rate drops. 
We observe important feedback coming from the BH, as for the Jiang case, green solid line, and also the BH has comparable mass. After this first efficient episode, the BH evacuate the surrounding region and $ \dot m$ drops. Subsequently the lower feedback at $f_E$ promote star formation and BH accretion is quenched, similar to J1e-3. %In the left lower panel of Fig. \ref{fig:snapa02}, we observe the temperature profile and the hot bubbles heated by the BH activity at the first timestep, which instead decrease after $0.38$ Myr (see Fig. \ref{fig:snapa02}). 
Thereafter, with the exception of a few episodes of SE accretion, the gas accretion rate follows a declining trend and - because $f_E < 1$ - the radiative efficiency is very similar to J1e-3 (see the red dashed and green lines in the lower panel of Fig. \ref{fig:1e3}), being - on average - larger than M1e-3 when $t < 0.2$ Myr, and smaller thereafter. The lower radiative efficiency favours star formation, quenching BH accretion. As a result, the time evolution of the BH mass in Ma01e-3 is closer to J1e-3 than to M1e-3, reaching a final value of $1300 M_{\odot}$. 

It is interesting to compare these findings with the results of Ma01e-6. The right panel of Fig. \ref{fig:1e3} shows that
when $\epsilon_c = 10^{-6}$, the effects of BH feedback are negligible and - despite the different values of $\epsilon_r$ - the three models follow a very similar time evolution, leading to similar final BH masses ($\sim 20000M_{\odot}$ for Ma01e-6).
We observe that BH feedback does not play a role and, after $0.4$ Myr, the disk configuration is the same as in M1e-6. %In the right panels of Figs. \ref{fig:snapa01} and \ref{fig:snapa02}, we observe that BH feedback does not play a role and, after $0.4$ Myr, the disk configuration is the same as in M1e-6. 
{\bf Fede: sono arrivata qua, devo rimuovere anche queste figure e compattarle nei grafici precedenti}
The dependence on the adopted BH spin of the time evolution of gas and stellar density radial profiles predicted in slim disk model is presented in Fig. \ref{fig:densa0}, for $\epsilon_c = 10^{-3}$ (left panel) and $10^{-6}$ (right panel). As expected, the dependence on BH spin is negligible when $\epsilon_c = 10^{-6}$. However, when $\epsilon_c = 10^{-3}$ we find that the two models show differences in the stellar density profile (when $t \geq 0.4$ Myr) and in the gas density profile (when $t > 0.4$ Myr) in the inner region of the disk, at $r < 2 - 3$ pc. These differences are reflected in the time evolution of the global star formation rate, which is systematically larger in Ma01e-3 than in M1e-3 beyond $t \sim 0.1$ Myr, while it has a similar trend in models M1e-6 and Ma01e-6. In all cases, the differences do not reflect in the time evolution of the total stellar mass, which appears to be insensitive to BH feedback (see Fig. \ref{fig:SFMstar}).
